# Supplementary material for: Lake Ice Detection from Sentinel-1 SAR with Deep Learning
Source: arXiv:2002.07040 source file (2020-05-06)
Supplement: Supplementary file 1 [file section7_appendices.tex]

\section{CONCLUSION AND OUTLOOK}

\begin{table}[]
    \small
    \caption{Per-class- and mean IoU values of frozen and non-frozen classes across winters (2016-17 and 2017-18). Data from all the three lakes St. Moritz, Silvaplana, and Sils on non-transition dates}
    \vspace{-0.5em}
    %\caption{A}
    %\hspace{-2em}
    \centering
     \begin{tabular}{|c|c|c|}
        \hline
        \diagbox[width=8em]{IoU}{Session} & 2016-17 & 2017-18  \\ \hline
        Non-frozen & 91.0\% & 90.0\%\\
        %\hline
        Frozen & 90.6\% & 87.7\%   \\
        \hline
        \textbf{Mean} & 90.8\% & 88.9\% \\
        \hline
    \end{tabular}
\end{table}
\normalsize
